# Supplementary material for: Stellar Signatures of Inhomogeneous Big Bang Nucleosynthesis
Source: arXiv:2006.02446 ancillary file (2020-06-03)
Supplement: Supplementary file 1 [file supplemental.pdf]

CERN-TH-2020-067

# Stellar Signatures of Inhomogeneous Big Bang Nucleosynthesis Supplemental Material

Alexandre Arbey*
*Univ Lyon, Univ Claude Bernard Lyon 1, CNRS/IN2P3,*
*IP2I Lyon, UMR 5822, F-69622, Villeurbanne, France*
*Theoretical Physics Department, CERN, CH-1211 Geneva 23, Switzerland and*
*Institut Universitaire de France (IUF), 103 boulevard Saint-Michel, 75005 Paris, France*

Jérémy Auffinger†
*Univ Lyon, Univ Claude Bernard Lyon 1, CNRS/IN2P3,*
*IP2I Lyon, UMR 5822, F-69622, Villeurbanne, France*

Joseph Silk‡
*Sorbonne Université, CNRS, UMR 7095, Institut dAstrophysique de Paris, 98 bis bd Arago, 75014 Paris, France*
*Department of Physics and Astronomy, Johns Hopkins University, Baltimore MD 2218, USA and*
*Beecroft Institute of Particle Astrophysics and Cosmology, University of Oxford, Oxford OX14BN, UK*
(Dated: June 3, 2020)

The data produced with `AlterBBN` [1, 2] for large values of the baryon-to-photon ratio $\eta$ are provided as supplemental material. The table `AlterBBN_data.out` contains the data in raw text format (with in addition larger values of $\eta$, which led to much larger uncertainties on the predicted abundances and were disregarded for our analysis), and the table `AlterBBN_data_reduced.out` contains the data reduced to the nuclei that play a significant role in high-$\eta$ BBN (see main paper). The figures 1 and 2 give the abundances of the elements as computed with `AlterBBN` for $\eta \in [10^{-10}, 10^{-1}]$, for each isotope as well as for the sum over all isotopes of each element. One panel is dedicated to each element. The solar abundances of [3] are given for comparison when available as red horizontal lines (the error bars are smaller than the width of the line). The vertical grey line corresponds to the Standard BBN value of $\eta = (6.104 \pm 0.058) \times 10^{-10}$ [4] (the error bars are smaller than the width of the line). The $y$-axis is a logarithmic scale of the abundances relative to a fixed hydrogen abundance of $10^{12}$. In the same format, we also present the `AlterBBN` data relative to Europium in Fig. 3, as this element is of utmost importance for the $r$-process enhancement evidence in dwarf galaxies [5, 6]. The Europium abundance did not pass the selection filters because of its very small value even in the high-$\eta$ scenarios considered here, but we provide its abundance here for completeness.

[1] A. Arbey, Comput. Phys. Commun. **183**, 1822 (2012), arXiv:1106.1363 [astro-ph.CO].
[2] A. Arbey, J. Auffinger, K. P. Hickerson, and E. S. Jenssen, Comput. Phys. Commun. **248**, 106982 (2020), arXiv:1806.11095 [astro-ph.CO].
[3] M. Asplund, N. Grevesse, A. J. Sauval, and P. Scott, Annu. Rev. Astron. Astrophys. **47**, 481 (2009), arXiv:0909.0948 [astro-ph.SR].
[4] B. D. Fields, K. A. Olive, T.-H. Yeh, and C. Young, J. Cosmol. Astropart. Phys. **2020**, 010 (2020), arXiv:1912.01132 [astro-ph.CO].
[5] A. P. Ji, A. Frebel, J. D. Simon, and A. Chiti, Astrophys. J. **830**, 93 (2016), arXiv:1607.07447 [astro-ph.GA].
[6] DES Collaboration, Astrophys. J. **882**, 177 (2019), arXiv:1812.01022 [astro-ph.GA].

* alexandre.arbey@ens-lyon.fr
† j.auffinger@ipnl.in2p3.fr
‡ joseph.silk@physics.ox.ac.uk

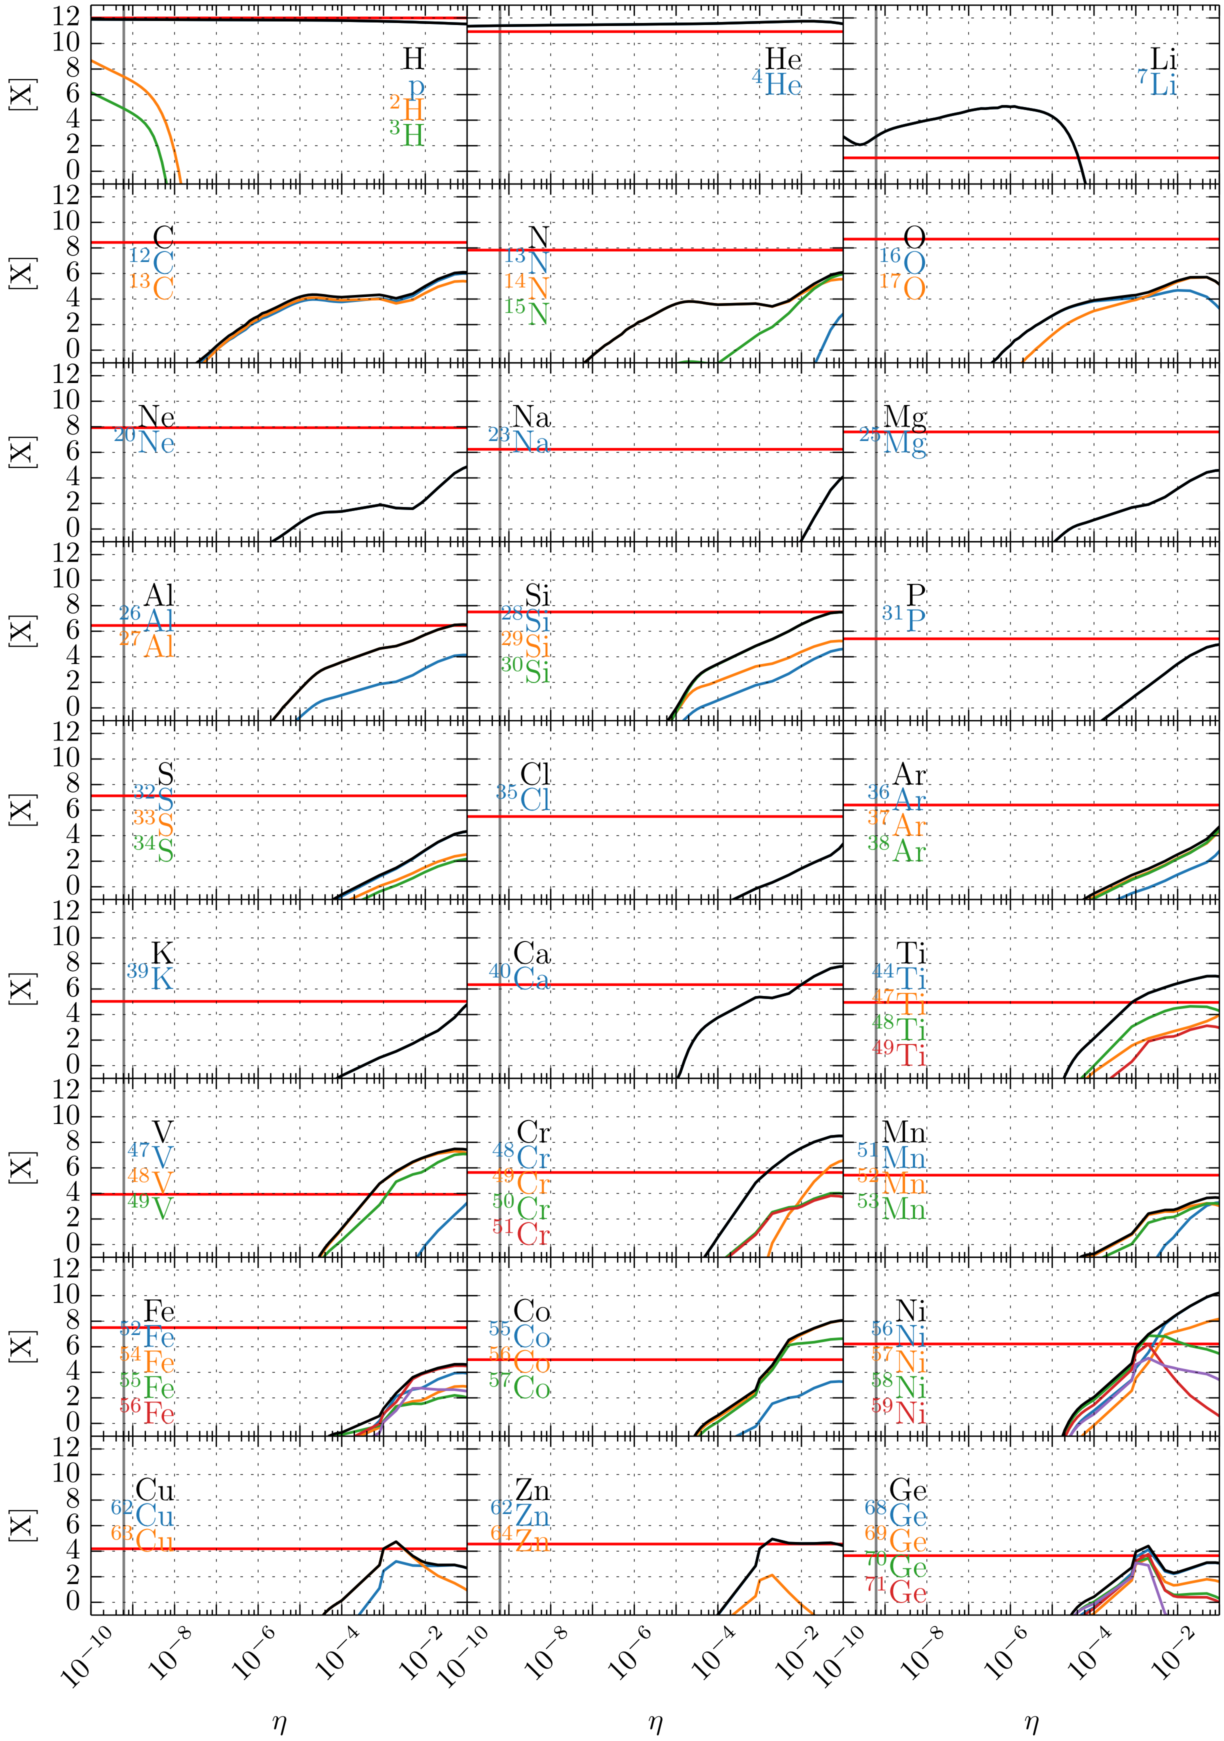


FIG. 1. Abundances of the elements computed with `AlterBBN` (plain curves) as functions of $\eta$ and compared to the solar abundances of [3] (when available, horizontal red lines). The SBBN value of $\eta$ of [4] is shown as a vertical grey line. Error bars are smaller than the width of the lines.

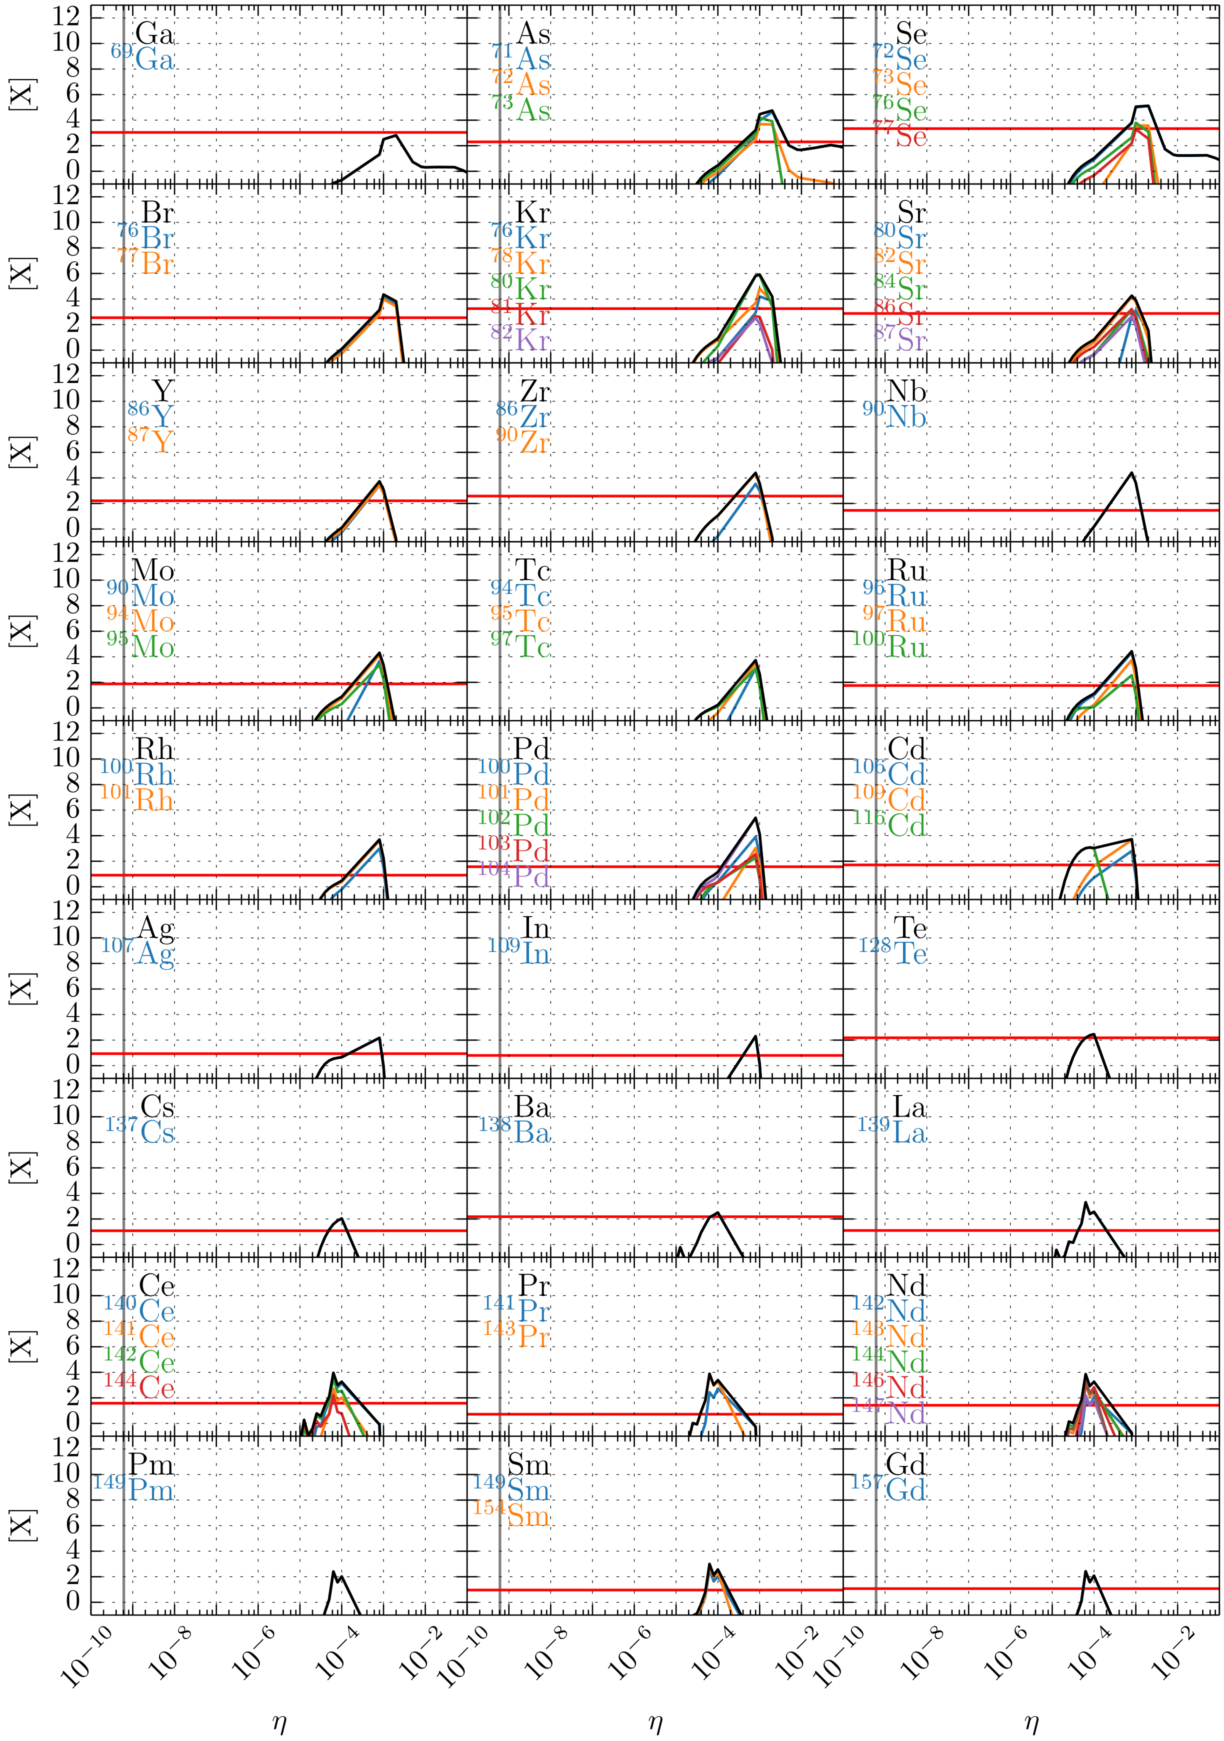


FIG. 2. Abundances of the elements computed with `AlterBBN` (plain curves) as functions of $\eta$ and compared to the solar abundances of [3] (when available, horizontal red lines). The SBBN value of $\eta$ of [4] is shown as a vertical grey line. Error bars are smaller than the width of the lines.

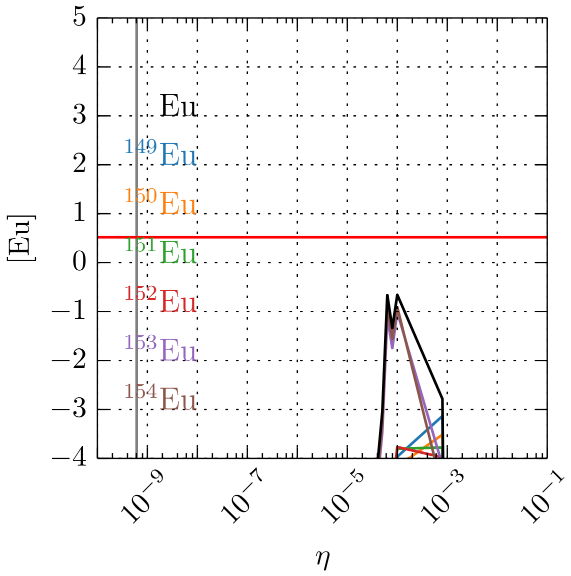


FIG. 3. Abundances of Europium computed with `AlterBBN` (plain curves) as functions of $\eta$ and compared to the solar abundance of [3] (horizontal red line). The SBBN value of $\eta$ of [4] is shown as a vertical grey line. Error bars are smaller than the width of the lines.
